# Supplementary material for: Refining 6-DoF Grasps with Context-Specific Classifiers
Source: arXiv:2308.06928 source file (2023-08-14)
Supplement: Supplementary file 1 [file appendix.tex]

\section{Appendix}

\subsection{GraspFlow: Additional Details}
\label{app:graspflow}
\rev{Pseudo-code for \method{} is shown in Algorithm \ref{alg:graspflow}. In practice, multiple grasps may be refined as a batch. 

\begin{algorithm}
\caption{\method}
\begin{algorithmic}[1]
\REQUIRE $f$-divergence and first derivative $f'$, grasp sampler $q_0$,  classifiers $p(c_i=1|\grasp, \obs)$, number of update steps ($N$) , step size ($\eta$), noise factor ($\gamma$).
\STATE $\rvg_{0} \sim q_0$ \algorithmiccomment{Initial grasp. Note: the sampler may be conditioned upon the context.}
\FOR{$n \gets 0$ to $N$}
    \STATE $\bm{\xi}_n \sim \mathcal{N}(0,I)$

    \STATE $\rvg_{n+1} = \rvg_{n} + \eta\nabla_\rvg \sum_i \log p(c_i | \grasp_n, \obs) + \sqrt{2\gamma\eta}\bm{\xi}_{n}$
\ENDFOR
\RETURN $\rvg_{n}$ \COMMENT{Refined grasp}
\end{algorithmic}
\label{alg:graspflow}
\end{algorithm}
}

\paragraph{Corrector Term.} 
Since the classifiers $p(c_i|\grasp, \obs)$ are not trained to distinguish samples from $q$ and $p$, a corrector term can be used to amend the flow and potentially improve refinement. We can train a discriminator to distinguish between samples drawn from $q$ (with label $\hat{d} = 1$) and the data used to train the criteria classifiers (grasps that do not satisfy all the specified criteria are labelled with $\hat{d} = 0$). Then, we can apply the correction, 
\begin{align}
\begin{split}
	\frac{q_{\tau_n}(\rvg_{\tau_n})}{p(\rvg_{\tau_n})} & = \frac{q_{\tau_n}(\rvg_{\tau_n})}{\hat{p}(\rvg_{\tau_n})}\frac{\hat{p}(\rvg_{\tau_n})}{p(\rvg_{\tau_n})} \\
 & \approx \frac{p(\hat{d}=1| \rvg_{\tau_n}, \obs)}{1-p(\hat{d}=1| \rvg_{\tau_n}, \obs)} \frac{1 - \prod_i p(c_i = 1 | \rvg_{\tau_n}, \obs)}{\prod_i p(c_i = 1 | \rvg_{\tau_n}, \obs)} \label{eq:correction}
\end{split}
\end{align}  
However, we did not find it necessary to apply this corrector; in preliminary trials, it did not provide significant improvement and requires access to the data (or sampling distributions) associated with the individual classifiers. 

\paragraph{Computation Time.} Compared to MH sampling, \method{} incurs additional computational cost to compute the gradients. In general, the computational cost of graspflow to refine a grasp candidate is $O(Tc)$ where $T$ is the number of time-steps and $c$ is the cost of computing the gradients in Eqn. \ref{eq:graspflow}.

\paragraph{6DOF Grasp Pose Refinement.} In our 6DOF grasp synthesis experiments, we represented each hand pose by its rotation and translation in $SE(3)$. The translation portion is handled in a straightforward manner. The pose orientation is handled similar to GraspNet~\cite{mousavian20196}; we sample a grasp candidate orientation as a quaternion, and convert it to Euler angle representation before refinement. After refinement, we convert the pose back to a quaternion for input to MoveIt!. A technical issue is regarding sampling of the noise term $\bm{\xi}_{\tau_n}$. The normal distribution  may differ depending on the representation of the grasp. For example, the normal distribution in $SO(3)$ differs from the Euclidean space~\cite{nikolayev1970normal}. In our implementation, we sampled directly from the standard normal distribution in Euclidean space\footnote{A similar approach was used in the GraspNet MH algorithm.}. While this is not technically correct, it worked well in our experiments. Future work can look into comparing whether more precise sampling results in better refinement.

\subsection{Grasp Stability Network}
\label{app:graspnetwork}

For the Stability discriminator, we used the same network architecture as GraspNet~\cite{mousavian20196}. Our robust classifier was trained using the following loss function:
\begin{align}
\begin{split}
    \mathcal{L}&=\left[- \frac{\alpha_1}{N}\sum_i^N \left(s_i\log(\hat{s}_i) + (1-s_i)\log(1-\hat{s}_i)\right)\right] \\
    & + \left[  \frac{\alpha_2}{N}\sum_i^N(\mathbf{t}_i-\hat{\mathbf{t}}_i)^2\right]\\
    & + \left[\frac{\alpha_3 }{N} \sum_i^N 2d_{\mathbf{r}_i}^2(4-d_{\mathbf{r}_i}^2)\right]
\end{split}
\end{align}

where $d_{\mathbf{r}_i}=\min(|\mathbf{r}_i-\hat{\mathbf{r}}_i|, |\mathbf{r}_i+\hat{\mathbf{r}}_i|)$. The loss can be seen as a composition of three terms, corresponding to the stability prediction ($s_i$), the reconstruction of the pose translation ($\mathbf{t}_i$), and rotation ($\mathbf{r}_i$). The hat notation denotes the model's predictions. The rotation is represented as a quaternion and the last term is the chordal loss~\cite{peretroukhin2020smooth}. In our experiments, we set $\alpha_1=0.85$, $\alpha_2=0.149$, and $\alpha_3=0.001$. \rev{We tuned the weights for each term manually; they were initially set to be equal and reduced such that each of the loss terms decreased at a similar rate. This was done to prevent overfitting on a validation set.}
The classifier was trained using Adam optimizer (learning rate = 0.0001) for 100 epochs.

\subsection{Comparison against MH Variants}
\label{sec:mh_variants}

\rev{
\begin{algorithm}
\caption{Grasp refinement with the  Metropolis-Hastings algorithm used in GraspNet}
\begin{algorithmic}[1]
\REQUIRE grasp sampler $q_0$,  classifiers $p(c_i=1|\grasp, \obs)$, number of update steps ($N$), sampling coefficient $\mathbf{c_g}$.
\STATE $\rvg_{0} \sim q_0$ \algorithmiccomment{Initial grasp}
\FOR{$n \gets 0$ to $N$}
    \STATE $\Delta_g \sim \mathcal{U}(-1,1)$ % this U is (-1,1)
    \STATE $\rvg^c = \rvg_{n} + c_g\Delta_g$
    \STATE $\alpha = \frac{p(c_i=1|\rvg^c, \obs)}{p(c_i=1|\rvg_{n}, \obs)}$
    \STATE $u \sim \mathcal{U}(0,1)$ % this one is (0,1)
    \IF{$u \leq \alpha$}
        \STATE $\rvg_{n+1} = \rvg^c$
    \ELSE
        \STATE $\rvg_{n+1} = \rvg_{n}$
    \ENDIF
\ENDFOR
\RETURN $\rvg_{n}$ \COMMENT{Refined grasp}
\end{algorithmic}
\label{alg:mh}
\end{algorithm}
}

We performed additional comparisons against variants of the Metropolis-Hastings (MH) method (\rev{Algorithm \ref{alg:mh}})\footnote{See: \url{https://github.com/NVlabs/6dof-graspnet}.}. The experimental setup follows Sec.  \ref{sec:graspflow6dof} and uses the Isaac Gym simulator to assess grasp success. Recall that the MH method refines 5000 sampled grasps for 135 iterations. We created two variants: MH-v1 which refines 20,000 samples for 135 iterations, and MH-v2 which refines 5000 samples for 500 iterations. Gradient computation was disabled for the MH methods. 

Fig. \ref{fig:mh_comparison} below shows the relative improvement provided by these two variants (applied to samples drawn from the GraspNet VAE). We have also included  \method{} and the original MH methods for  comparison. Note that for MH-v1, we scored the top 5000 grasps (after sampling) using the classifier and report success performance using the simulator so that the relative improvement scores are comparable across methods. We also show MH-v1a where  performance was reported over all 20k grasps. 

Among the MH variants, MH-v2 performs the best. The MH-v2 performance approaches that of \method{}, which is expected since it also benefits from the robust classifier. However, MH-v2 requires significantly more computation time. MH-v2 takes an average of 1435 seconds to refine 5000 grasps over 500 iterations (compared to \method{}, which takes an average of 438 seconds to refine 5000 grasps over 50 iterations). These results support the notion that gradients provide useful information for refinement, allowing good samples to be obtained with lower computational cost. 

\begin{figure}
    \centering
    \includegraphics[width=\linewidth]{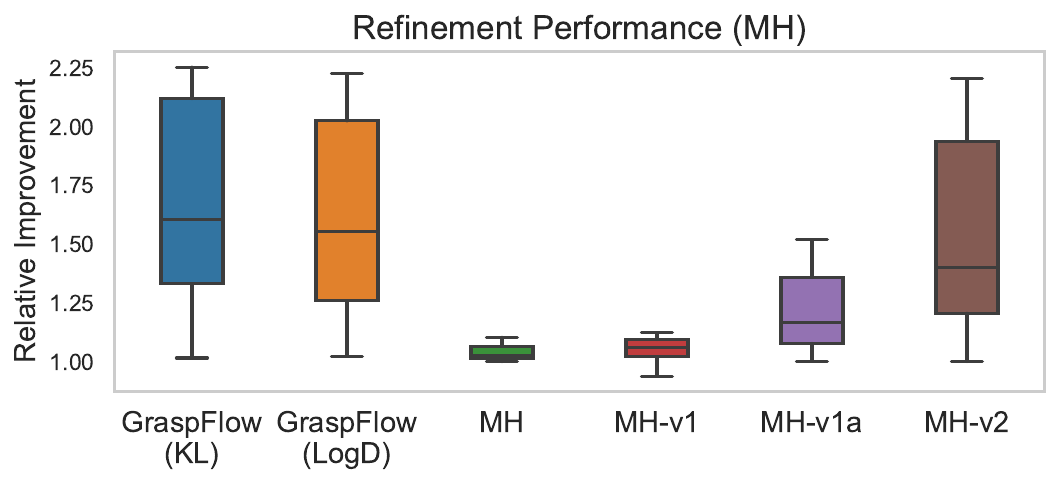}
    \caption{Comparison against two additional MH variants. Recall that MH refines 5000 grasps for 135 iterations. MH-v1 refines 20,000 grasp samples for 135 iterations and MH-v2 refines 5000 samples for 500 iterations. In all three cases, refinement was performed using the robust classifier.}
    \label{fig:mh_comparison}
\end{figure}
